# Supplementary material for: BYE: Build Your Encoder with One Sequence of Exploration Data for Long-Term Dynamic Scene Understanding
Source: arXiv:2412.02449 source file (2024-12-03)
Supplement: Supplementary file 1 [file 7_appendix.tex]

% \section*{APPENDIX}
\clearpage
\appendix
\section{Per-Class Object Association Results Visualization}
\begin{figure}[h]
\centering
\includegraphics[width=0.49\textwidth]{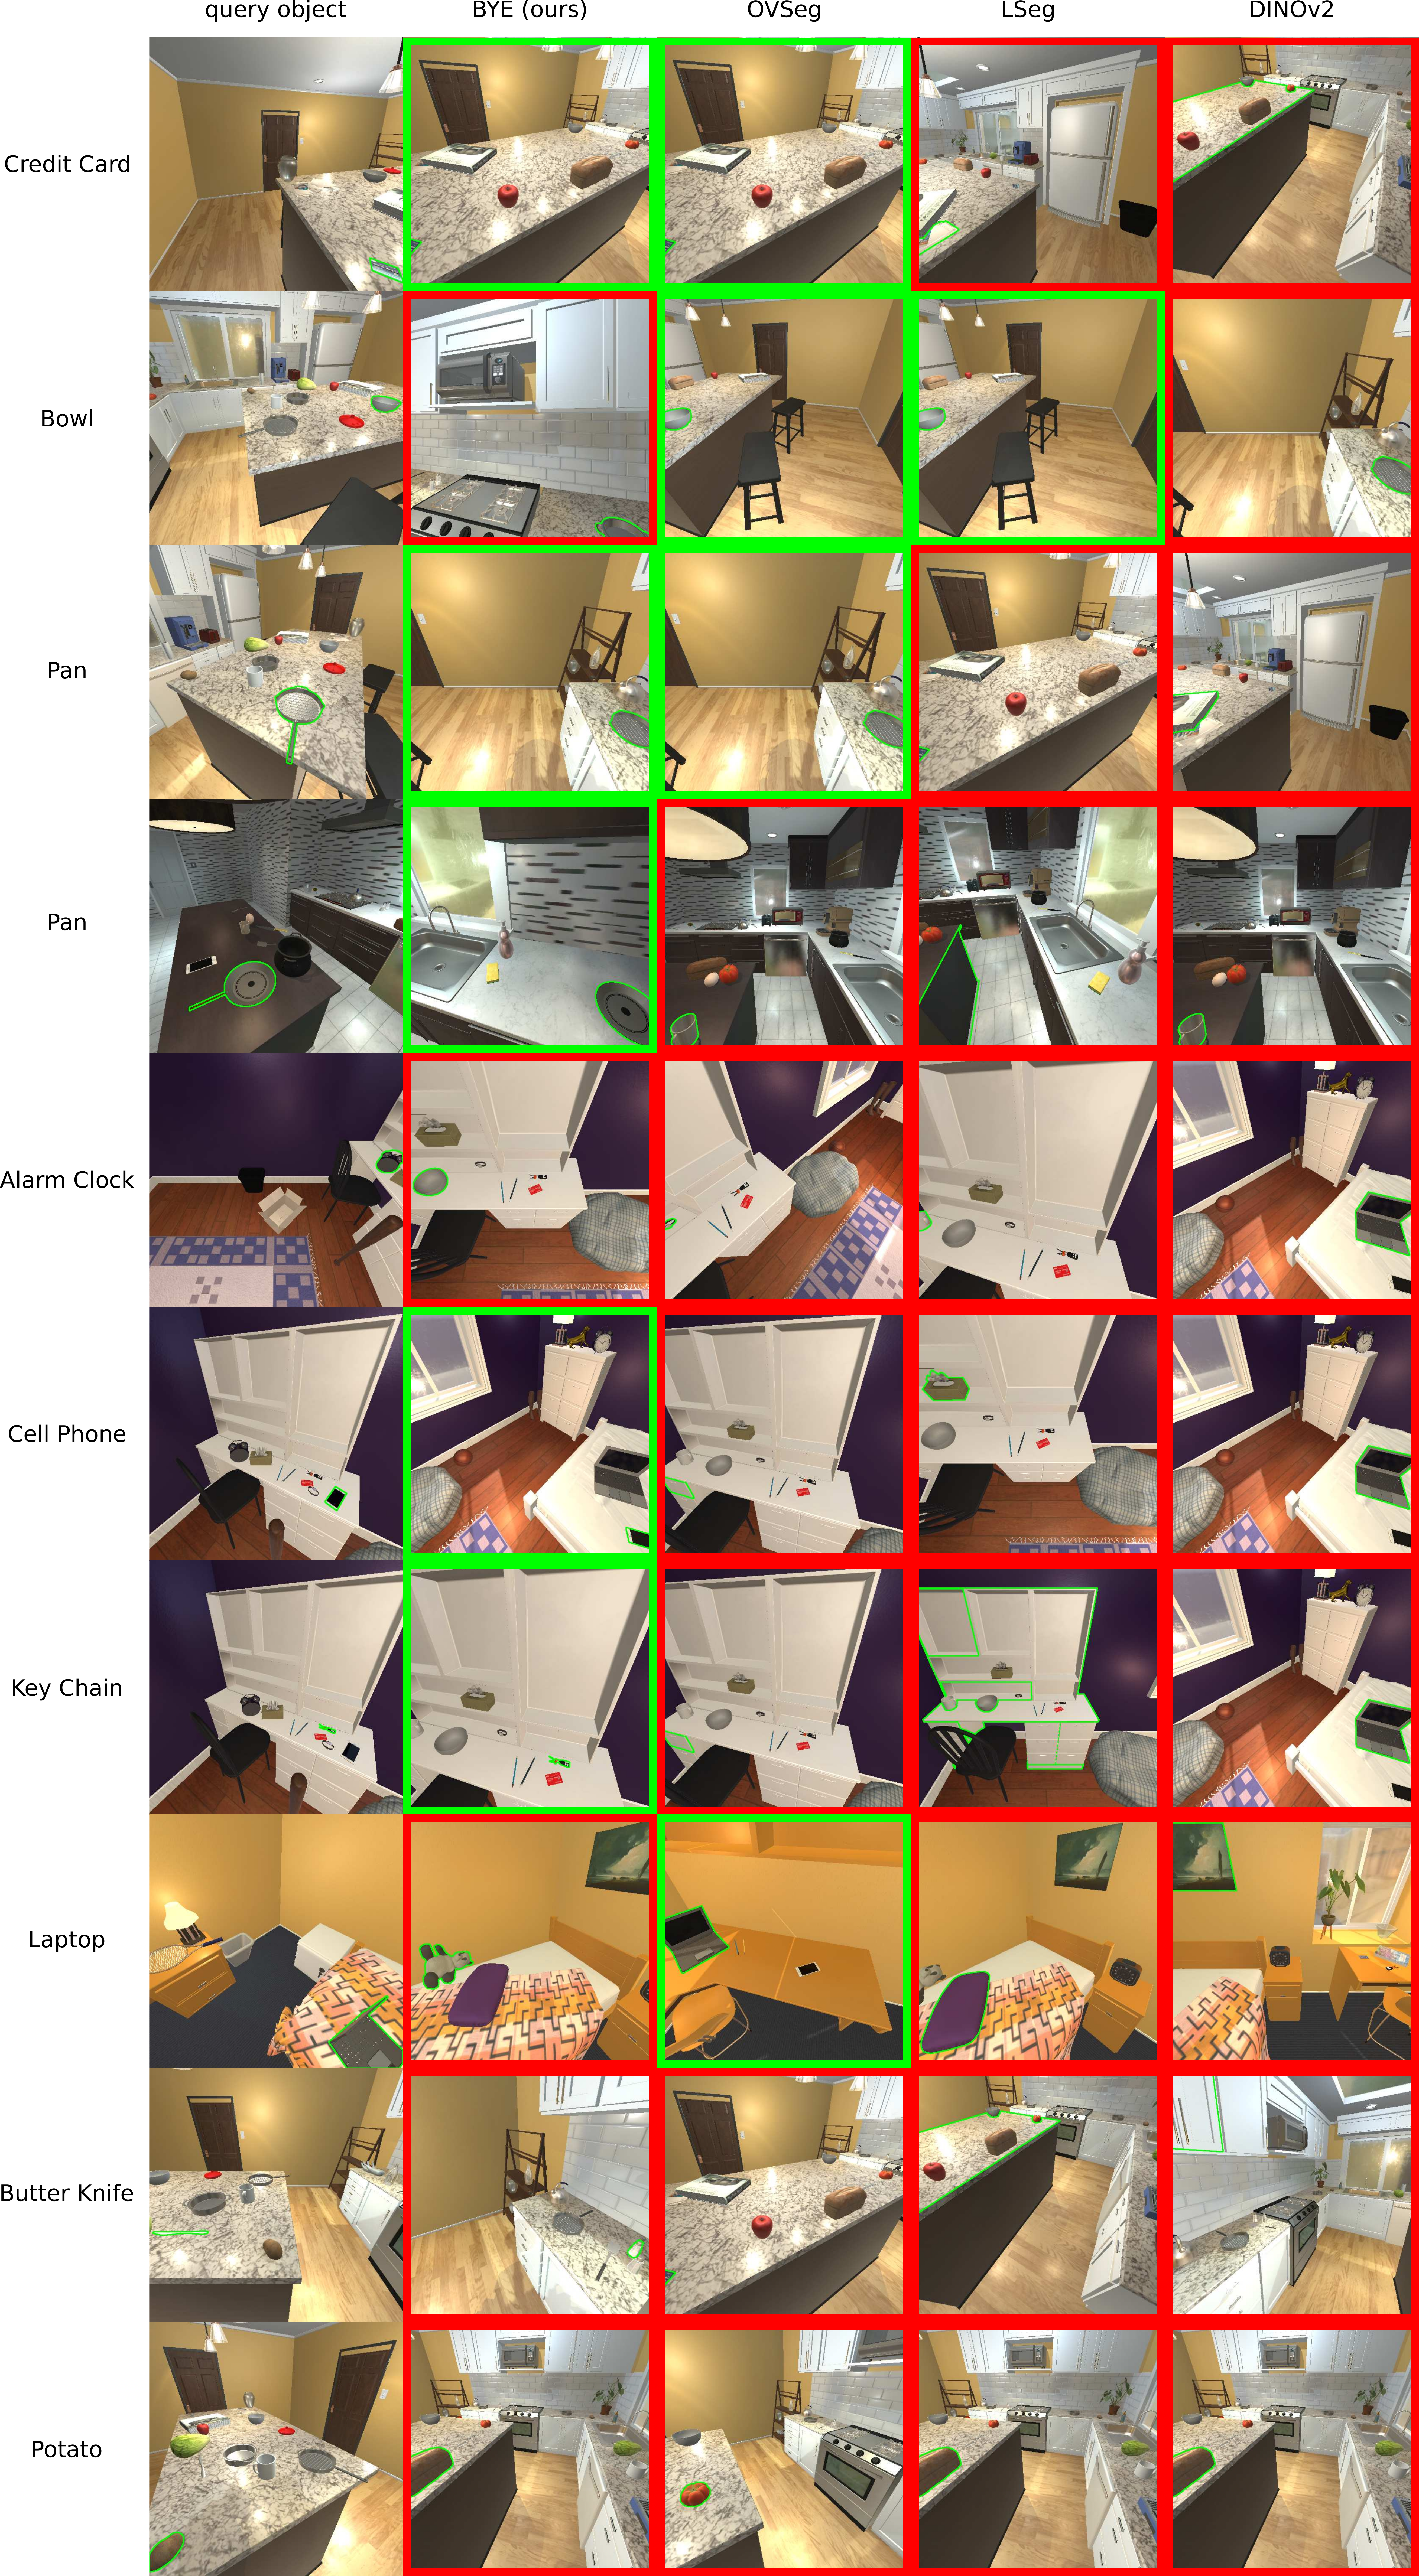}
\caption{Per-class object association qualitative results in AI2THOR.}
\label{fig:per_class_visualization}
\end{figure}

\section{Per-Scene Association Success Rates}

We show the per-scene association success rates in Fig.~\ref{fig:recall_per_scene}.

\begin{figure}[h]
\centering
\includegraphics[width=0.49\textwidth]{images/recall_per_scene.png}
\caption{The association success rate in each tested scene in AI2THOR.}
\label{fig:recall_per_scene}
\end{figure}

\section{Evaluated Scenes in AI2THOR}
\label{sec:evaluated_scenes_ai2thor}
We evaluated FloorPlan 1, 2, 4, 5, 6, which are kitchens, and FloorPlan 301-305, which are bedrooms.
